# Supplementary material for: MagicVideo: Efficient Video Generation With Latent Diffusion Models
Source: arXiv:2211.11018 source file (2023-05-11)
Supplement: Supplementary file 1 [file _supp.tex]

\section{Preliminary}
\subsection{Generative Modeling through Diffusion Models}
% \paragraph{Denoising Diffusion Probabilistic Models}
% Deep generative modeling utilizes neural networks to approximate the distribution from which the training data are sampled.
Denoising diffusion probabilistic models (DDPM) approximate the probability densities of training data via the reversed processes of Gaussian diffusion processes \cite{ho_denoising_2020}, where deep neural networks parameterize the transition dynamics that progressively remove noise and synthesize clean samples. 

DDPMs have achieved great success in image generation~\cite{ho_denoising_2020, song_score-based_2021} and editing \cite{lugmayr_repaint_nodate, meng_sdedit_2022, hertz_prompt--prompt_2022, liew_magicmix_2022, kawar_imagic_2022}. However, due to the large step number of iterations during sampling, the computational overhead of DDPMs gets very high and impedes their applications. To improve the efficiency of DDPMs, researchers have developed several advanced sampling methods by utilizing high-order SDE/ODE solvers~\cite{song_score-based_2021, lu_dpm-solver_2022, song_denoising_2022}, and also have explored novel diffusion-based modeling methods. Rombach \etal~2022~\cite{rombach_high-resolution_2022} proposed the latent diffusion model (LDM) that models the data distribution in a low-dimensional latent space. Denoising noisy data in a lower dimension may reduce the computational cost in the generation process. Vahdat \etal~2021~\cite{vahdat_score-based_2021} concurrently proposed a latent score-based model that shares similar ideas with LDM. 

Specifically, LDM first trains an autoencoder $\mathcal{E}$-$\mathcal{D}$ to map images $\vx$ into a low-dimensional space and reconstruct images from latent codes $\vz$. Then, the autoencoder is jointly trained with a perceptual loss and a patch-based adversarial objective. This training scheme ensures the spatial correspondence between latent codes and the original images.
Then, a DDPM with a time-conditional U-Net backbone is used to model the distribution of the latent representations. To enable controllable/conditional generation, LDM uses a domain-specific encoder $\tau(\cdot)$ to project the control signal $\vy$ (\eg a text prompt) into an intermediate space and subsequently injects the embedding into the U-Net via a cross-attention layer. The implementation of the VAE is inspired by the LDM and based on the public stable-diffusion\footnote{Stable-Diffusion: \url{https://huggingface.co/CompVis/stable-diffusion}} code base.  

\subsection{Video Generation}
Researchers have explored various video generation methods in the past several years, including using GAN-based \cite{vondrick_generating_2016, clark_adversarial_2019, tulyakov_mocogan_2017} and auto-regressive methods to model the distributions \cite{ranzato_video_2016, kalchbrenner_video_2017, babaeizadeh_fitvid_2021, kumar_videoflow_2020, mathieu_deep_2016, hong_cogvideo_2022} of video frames in RGB or latent spaces. Recently, diffusion-based generative models have shown excellent performance for (conditional) image generation, which triggers significant interest in exploring their applications in video modeling. Ho \etal  \cite{ho_video_2022} present a natural extension of the vanilla DDPM for image generation to the video domain. They proposed a 3D U-Net diffusion model architecture and a novel conditional sampling technique for longer video generation. Harvey \etal  \cite{harvey_flexible_2022} propose to model the conditional distribution of subsequent video frames given certain observed ones so that a long video can be synthesized by conditional sampling in an auto-regressive manner. Similarly, Yang \etal  \cite{yang_diffusion_2022} propose a two-step framework for video generation\textemdash using a deterministic model to predict the next frame given observed ones, then utilizing a stochastic diffusion model to synthesize the residual for correcting the next frame prediction. 

In this work, we are interested in text-conditional video generation. Ho \etal \cite{ho_imagen_2022} proposed a cascaded pipeline, termed Imagen Video, to synthesize high-definition videos. The pipeline consists of one base text-to-video module, three spatial super-resolution (SSR), and three temporal super-resolution modules (TSR). The base text-to-video module utilizes temporal attention layers, while temporal convolutions are used in SSR and TSR modules. Concurrently, Singer \etal  \cite{singer_make--video_2022} propose a multi-stage text-to-video generation method, termed Make-A-Video. The proposed method exploits a text-to-image model to generate image embeddings, then trains a low-resolution video generation model with conditioning on the image embeddings, and finally trains spatial and spatial-temporal super-resolution models to synthesize high-definition videos. Both Imagen Video and Make-A-Video model the video distribution in the RGB space. Differently, our work explores a more efficient way for video generation by synthesizing videos in a low-dimensional latent space.
